# Supplementary material for: LEOPARD: Identifying Vulnerable Code for Vulnerability Assessment through Program Metrics
Source: arXiv:1901.11479 source file (2020-01-19)
Supplement: Supplementary file 1 [file sec08-appendix.tex]

% !TeX root = main.tex

\section{Supplementary Results}\label{sec:appendix}

In this section, we provide the supplementary results about the sensitivity analysis of vulnerability metrics in Fig.~\ref{fig:sensitivity2}.

\begin{figure*}[!t]
\centering

\begin{subfigure}[b]{0.33\textwidth}
\centering
\begin{minipage}{\linewidth}
\includegraphics[width=0.9\textwidth]{./figs/glibc_vd.pdf}
\end{minipage}
\caption{glibc 2.22}\label{fig:glibcVD}
\end{subfigure}
\begin{subfigure}[b]{0.33\textwidth}
\centering
\begin{minipage}{\linewidth}
\includegraphics[width=0.9\textwidth]{./figs/ffmpeg_vd.pdf}
\end{minipage}
\caption{ffmpeg 3.1.3 }\label{fig:ffmpegVD}
\end{subfigure}
\begin{subfigure}[b]{0.33\textwidth}
\centering
\begin{minipage}{\linewidth}
\includegraphics[width=0.9\textwidth]{./figs/qemu_vd.pdf}
\end{minipage}
\caption{QEMU 2.5.0}\label{fig:QEMUVD}
\end{subfigure}

\begin{subfigure}[b]{0.33\textwidth}
\centering
\begin{minipage}{\linewidth}
\includegraphics[width=0.9\textwidth]{./figs/asterisk_vd.pdf}
\end{minipage}
\caption{Asterisk 12.0.0}\label{fig:AsteriskVD}
\end{subfigure}
\begin{subfigure}[b]{0.33\textwidth}
\centering
\begin{minipage}{\linewidth}
\includegraphics[width=0.9\textwidth]{./figs/libxml2_vd.pdf}
\end{minipage}
\caption{libxml2 2.9.4}\label{fig:libxml2VD}
\end{subfigure}
\begin{subfigure}[b]{0.33\textwidth}
\centering
\begin{minipage}{\linewidth}
\includegraphics[width=0.9\textwidth]{./figs/libxslt_vd.pdf}
\end{minipage}
\caption{libxslt 1.1.28}\label{fig:libxsltVD}
\end{subfigure}

\begin{subfigure}[b]{0.33\textwidth}
\centering
\begin{minipage}{\linewidth}
\includegraphics[width=0.9\textwidth]{./figs/openssl_vd.pdf}
\end{minipage}
\caption{OpenSSL 1.0.1t}\label{fig:OpenSSLVD}
\end{subfigure}
\begin{subfigure}[b]{0.33\textwidth}
\centering
\begin{minipage}{\linewidth}
\includegraphics[width=0.9\textwidth]{./figs/wireshark_vd.pdf}
\end{minipage}
\caption{Wireshark 2.2.0}\label{fig:WiresharkVD}
\end{subfigure}
\begin{subfigure}[b]{0.33\textwidth}
\centering
\begin{minipage}{\linewidth}
\includegraphics[width=0.9\textwidth]{./figs/linux_vd.pdf}
\end{minipage}
\caption{Linux 4.8.11}\label{fig:LinuxVD}
\end{subfigure}
\vspace{-10pt}
\caption{Sensitivity Analysis Results of the Vulnerability Metrics}\label{fig:sensitivity2} 
\end{figure*}
